# Supplementary material for: Coulomb drag between carbon nanotube and graphene
Source: arXiv:1612.05992 ancillary file (2017-10-18)
Supplement: Supplementary file 1 [file Coulomb_drag_between_carbon_nanotube_and_graphene_Supp_Info.pdf]

# Coulomb drag between carbon nanotube and graphene - Supplementary information - Supplementary information

Jean-Damien Pillet[1,2], Austin Cheng[3], Takashi Taniguchi[4], Kenji Watanabe[4], Philip Kim[3]
[1]*Department of Physics, Columbia University, New York, New York 10027, USA.*
[2]*Laboratoire des Solides Irradiés, École Polytechnique, CNRS, CEA, Université Paris-Saclay, 91128 Palaiseau, France.*
[3]*Department of Physics, Harvard University, Cambridge, Massachusetts 02138, USA. and*
[4]*National Institute for Materials Science, Namiki 1-1, Ibaraki 305-0044, Japan.*

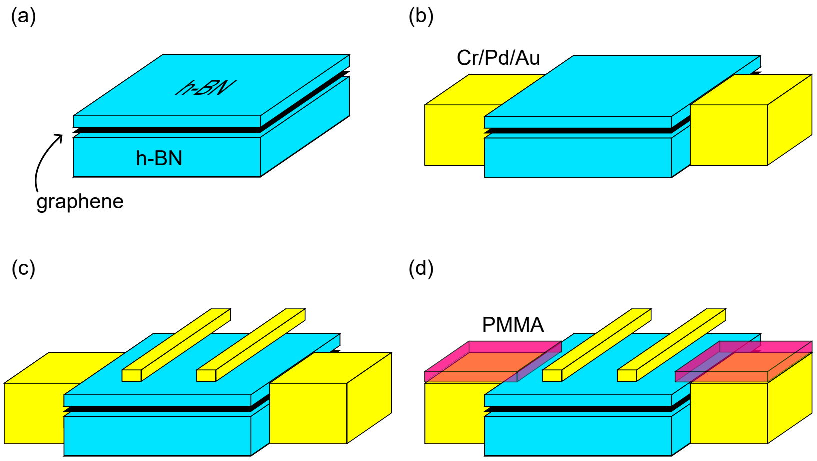


Figure S1. Sequence of preparation of the h-BN encapsulated graphene for nanotube transfer. (a) h-BN/graphene/h-BN sandwich. (b) The graphene is electrically connected after a first step of lithography using RIE in order to expose the edges of the graphene flake followed by a metallic evaporation. (c) Electrodes, electrically isolated from the graphene by the top layer of h-BN, are prepared for connection of the carbon nanotube. (d) The sample is partially covered with resist. It will help the subsequent incorporation of a carbon nanotube in the structure.

## I. FABRICATION

### A. Preparation of the circuit

The sample shown in Fig. 1 of the main text is based on the initial preparation of an h-BN encapsulated flake of graphene [1] (Fig. S1 (a)) on an n-doped silicon wafer with 285 nm SiO2. The thickness of the top h-BN layer is chosen between 5 and 15 nm and the bottom one around 40 nm. We use standard technique of e-beam lithography to design the electrodes contacting the graphene flake. We first expose the edges of the graphene flake by reactive ion etching through a resist mask and subsequently evaporate a metallic trilayer Cr(1nm)/Pd(15nm)/Au(30nm) through the same mask (Fig. S1 (b)). A second step of lithography is then performed to design electrodes (same metallic trilayer) on top of the top h-BN layer. These electrodes are used to contact the carbon nanotube during the transfer step described at the end of this section (Fig. S1 (c)). The sample is covered with a 100nm thick layer of resist (PMMA A4 495K) except for areas of interest where we want the nanotube to connect electrodes during transfer. The resist will help for an efficient transfer of the carbon nanotube (Fig. S1 (d)).

### B. Growth of nanotubes and characterization

Carbon nanotubes are grown and characterized following the techniques described in Ref. [2]. They are grown on $5 \times 5\text{mm}^2$ silicon chip with a slit in the center (see bottom of Fig. S2) using standard technique of chemical vapor deposition. A catalyst is deposited on one side of the slit (middle) such that carbon nanotubes grow suspended (top). One of these nanotubes, suspended over a slit that is 65$\mu$m wide and 1cm long, is shown in the optical picture of Fig. S2. It is covered with 30 nm of Au, so it can be seen optically.

After growth, carbon nanotubes can be characterized using Rayleigh scattering. This helps to identify whether nanotubes are metallic or semiconducting as illustrated in Fig. S3. Moreover it also allows to measure the position of the carbon nanotube along the slit such that it can be aligned with the circuit for subsequent transfer.

### C. Transfer

The incorporation of the carbon nanotube into the circuit is performed by mechanical transfer [3] similarly to what is done to make h-BN encapsulated graphene. The slit is placed above the circuit in order to align the nanotube with the area of interest where we have designed dedicated electrodes. The slit is pressed on the sample as shown in Fig. S4. When we have a good mechanical contact, we warm the chips up to 180°C during 5 minutes in order to melt the

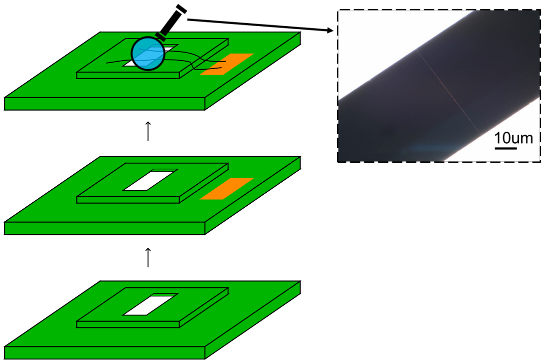


Figure S2. Sequence illustrating the growth of suspended carbon nanotubes.

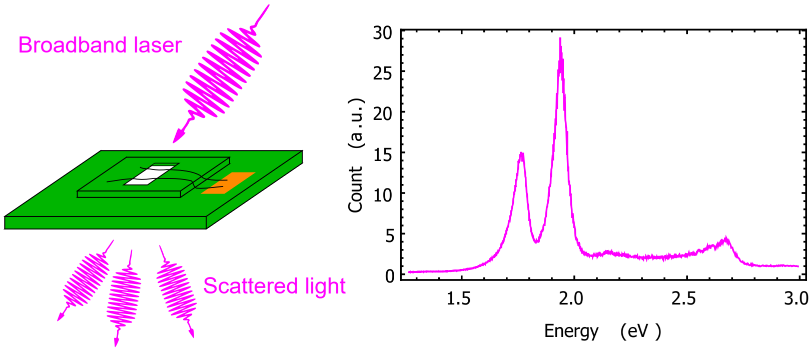


Figure S3. Rayleigh scattering. Carbon nanotubes are characterized when suspended over the slit. A broadband laser is sent through the light and the scattered light is collected with a detector (left). A typical spectrum is shown on the right, it gives the nanotube chirality. In this example the nanotube was metallic with a $(16, 4)$ chirality.

resist that will help the nanotube to be transferred from the slit to the target chip. The two chips are then slowly separated after they have cooled down to room temperature.

## II. PARASITIC CAPACITIVE EFFECT

Electrostatic cross-talk can be a major source of parasitic signal in Coulomb drag measurements. This cross-talk is generally mediated by unwanted capacitance in the setup and can be characterized by performing DC measurements (Fig 1 of the main) and frequency dependence measurements of the drag signal.

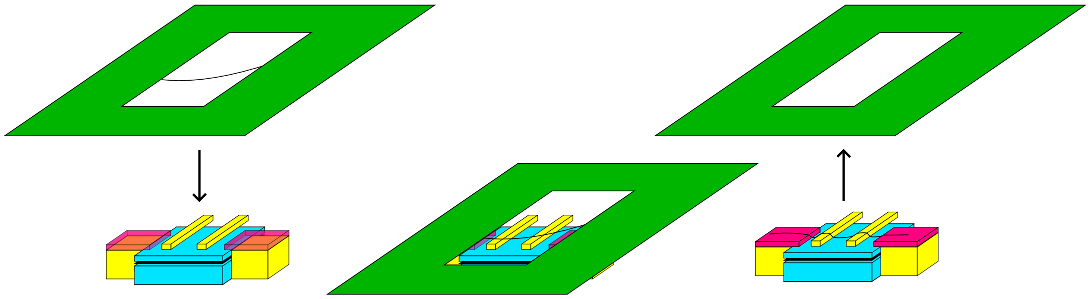

Figure S4. Sequence illustrating the nanotube transfer. The slit on which the nanotube is suspended is aligned with the h-BN encapsulated graphene (left). It is then pressed onto the target chip that is warmed up to 180°C in order to melt the resist and favor the transfer of the nanotube from one chip to another (center). The two chips are then separated from each other and the nanotubes is left onto its electrodes and over the h-BN/graphene/h-BN sandwich.

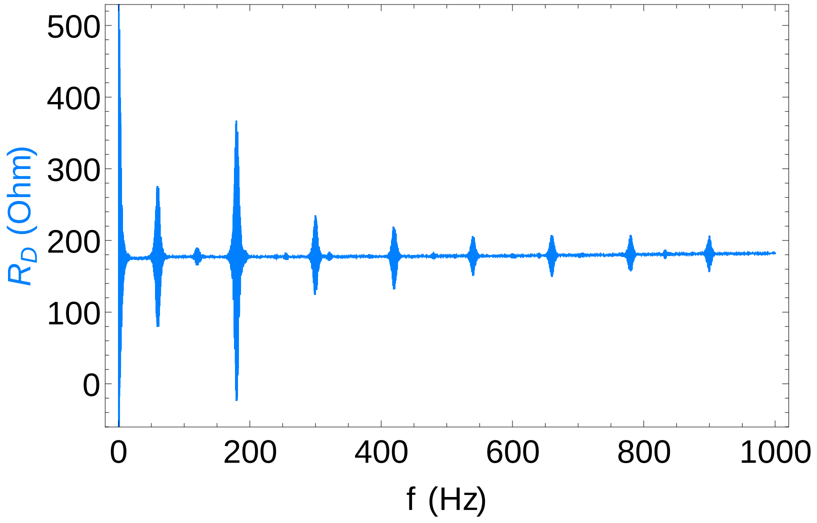


Figure S5. Drag resistance measured using a lock-in technique as a function of frequency. The mean value of $R_D$ only increase by a few percent between 0 and 1kHz indicating a weak capacitive contribution in the signal. The bursts of noise observed at multiple of 60 Hz are due to mains hum from the electric power supply.

The main reason for electrostatic parasitic signals is the capacitive coupling between the different layers of the device (nanotube and graphene) partially because of their shared capacitance (of the order of a few tens or hundreds of aF, limited by the size of the nanotube) but mainly because of the large capacitance C between the wires of the fridge (hundreds of pF up to a few nF). This can become problematic when we perform lock-in measurements at finite frequency $f$ if the samples have large resistance $R_{G(NT)}$ (respectively for graphene and nanotube) but small drag resistance $R_D$. Indeed, an AC current send to one layer will partially flow in the other layer by capacitive coupling and generate a parasitic signal.

The ratio of the drag signal over this parasitic one is given by $R_D/(2\pi f R_{NT} R_G C)$ which needs to remain as large as possible in order to detect Coulomb drag. Since the typical capacitance between wires of the fridge is a few hundreds of pF, the typical resistance is a few k$\Omega$ for graphene and a few tens of k$\Omega$ for nanotube, it means the frequency have to be negligible compared to $R_D$ x 1 Hz.Ohm-1. This makes lock-in measurements rather challenging if not impossible if $R_D$ is only a few Ohms (as in 2DEG at low temperature), however, in our case, we observe that $R_D$ is of a few hundreds of $\Omega$ for DC measurements which means that $f$ has to be lower than a few hundreds of Hz. As, we perform most of our measurements around 20 Hz, we are well below this limit and have no parasitic capacitive signal.

Moreover, one can easily discriminate a drag signal from a capacitive one as such parasitic contribution would be increasing with the frequency of the applied voltage (since sample and parasitic capacitance form a RC filter). We performed a frequency dependence measurements and observe no modulation of our signal with frequency (see Fig. S5). We can therefore rule out any parasitic signal in $R_D$ that would come from capacitive coupling between the layers or the wires of the fridge.

## III. CHARGE CARRIER DENSITY AND TEMPERATURE DEPENDENCE OF THE DRAG RESISTANCE

In Fig. 2b of the main text, we show the dependence of $R_D$ as a function of the back gate voltage $V_{bg}$. It shows a maximum that corresponds to te Dirac peak and then slowly goes toward zero following a power law as shown in Fig. S6. As $|V_{bg} - V_{Dirac}|$ is directly proportional the charge carrier density in graphene $n_G$, this means that $R_D \propto n_G^{\alpha}$ where $\alpha \approx -0.6$ according to the fit corresponding to the black dashed line. This has to be compared with the $n_G^{-2}$ dependence that has been observed previously in graphene-graphene Coulomb drag experiment.

Following Ref. [4], one can try to fit the evolution of $R_D$ with temperature by a power law $T^{\alpha}$ at high temperature and by an Arrhenius law $\exp(-T_1/T)$ at low temperature as shown in Fig. S7. Though we observe a similar trend, we cannot conclude about the microscopic implications in our system.

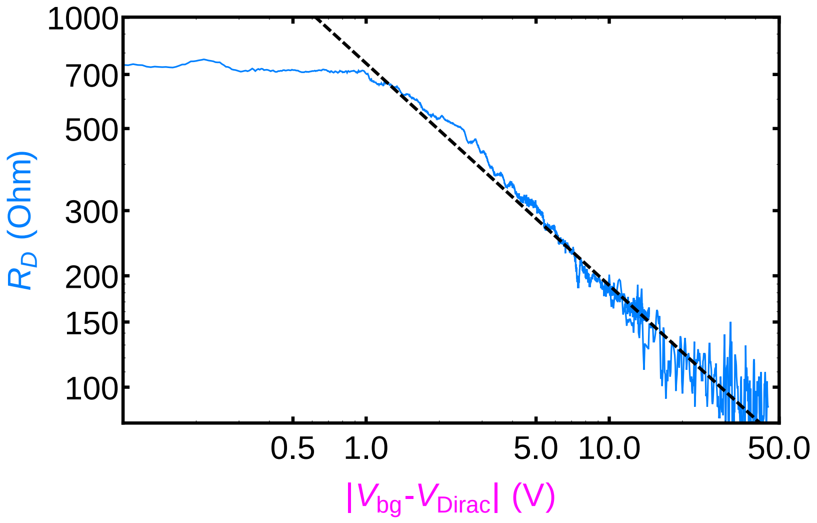


Figure S6. Dependence of the drag resistance with back gate voltage $V_{bg}$ or equivalently charge carrier density $n_G$ in the graphene flake (as $n_G \approx V_{bg} \times C_{SiO_2}/e$ where $C_{SiO_2}$ is the capacitance between graphene and back gate and $e$ is the charge of electron) in a log-log scale. Close to the Dirac peak centered at $V_{Dirac}$, $R_D$ saturates at a maximum value and then decreases toward 0 following a power law $n_G \propto |V_{bg} - D_{Dirac}|^{-0.6}$.

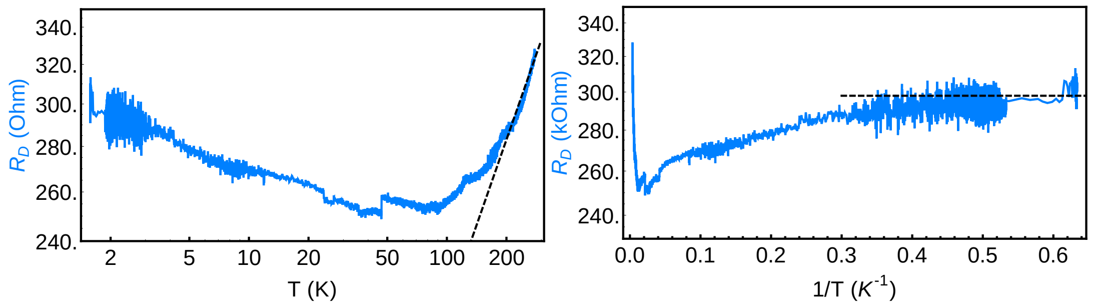


Figure S7. Temperature dependence of $R_D$ shown in Fig. 2 of the main text but this time presented in log scale as a function of temperature $T$ (left) and $1/T$ (right). The black dashed line on the left graph shows the power law $T^{0.4}$ and the one on the right shows the saturation of $R_D$ at large $1/T$ typical of an Arrhenius law.

## IV. BROADENING OF THE DIRAC PEAK IN GRAPHENE DUE TO THE PRESENCE OF NANOTUBE ELECTRODES

In the inset of Fig. 2b of the main text, we show the graphene resistance $R_G$ as a function of the back gate voltage $V_{bg}$. The Dirac peak looks much broader and less symmetric than the peak observed in $R_D$. The reason for this poorly defined peak is due to the presence of electrodes on top of the top h-BN layer that are designed to connect a carbon nanotube. Indeed, the presence of these electrodes causes the chemical potential to be inhomogenous in the graphene flake and may result in multiple appearances of the Dirac peak when measuring $R_G$ as a function of back gate voltage $V_{bg}$.

Fig. S8 shows the graphene resistance $R_G$ measured in a test-sample as a function of back gate voltage $V_{bg}$ and the voltage $V_{NTelec}$ applied on electrodes lying on top of the h-BN encapsulated graphene. On the top curve, we observe that the Dirac peak appears broad, irregular and asymmetric suggesting an imhomogenous chemical potential in the graphene flake. In the bottom graph, we can identify that this irregular peak is actually the superposition of two regular Dirac peaks: one corresponding to the part of the graphene flake that is locally gated by the nanotube electrodes with a position along the $V_{bg}$ axis depends on $V_{NTelec}$, and another one that corresponds to the rest of the flake and is not covered with nanotube electrodes.

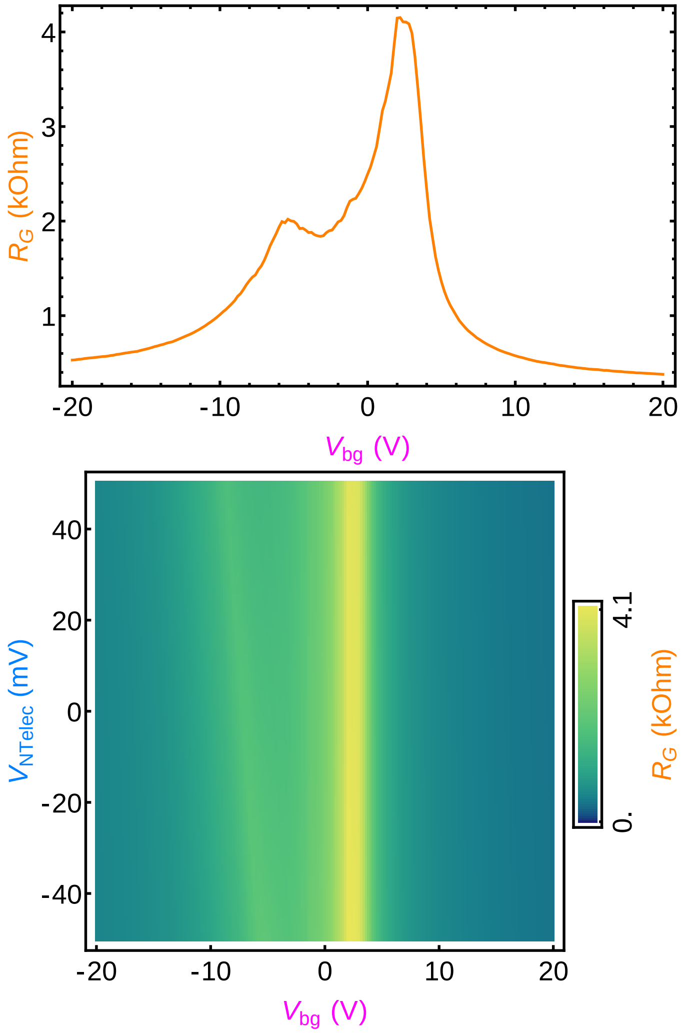


Figure S8. Graphene resistance of a test sample with electrodes lying on top of an h-BN encapsulated graphene flake. The Dirac peak can appear multiple times in $R_G$ depending on he voltage $V_{NTelec}$ applied on the electrodes designed for nanotube transfer. The top curve is measured at $V_{NTelec} = 50$ mV.

## V. GRAPHENE MAGNETO-RESISTANCE - ONSAGER RELATION

As can be seen in Fig. 2d and e of the main text, $R_D$ is not symmetric with the sign change of $B$, regardless of whether $R_D$ is measured across the nanotube or graphene. For a circuit with two terminals, this symmetry should be preserved as it would otherwise violate time-reversal symmetry. This apparent violation is due to the multiterminal measurement conguration of our drag experiments. Even when no current is flowing through the nanotube, its electrons might scatter with those of graphene which induces finite non-diagonal terms in the conductance matrix relating currents and voltages in the device. In this case, time-reversal symmetry dictates that $R_D$ should obey Onsager relations [5, 6] implying $R_D^G(B) = R_D^{NT}(-B)$, where $R_D^{G(NT)}$ is the drag resistance measured across graphene (resp. nanotube). As illustrated in Fig. 2f of the main text, our measurements obey such relations and time-reversal symmetry is not violated in our experiment, even at low temperature, in contrast with what has been reported previously in devices based on two-dimensional conductors [7, 8].

For a two-terminal measurement, $R_D(B) \neq R_D(-B)$ would imply a violation of Onsager relations [5] that originate from time-reversal symmetry. We can test this symmetry by measuring, for example, the two-terminal resistance of graphene $R_G$. This measurement is shown in Fig. S9 (a) and (b) as a function of $V_{bg}$ and $B$. We can see that it is symmetric with magnetic field.

For $R_D$, the conditions imposed by Onsager relations are different because we are performing a three-terminal measurement. However, as shown in Fig. S9 (c), we can symmetrize the drag resistance $R_D$ if we define the latter as

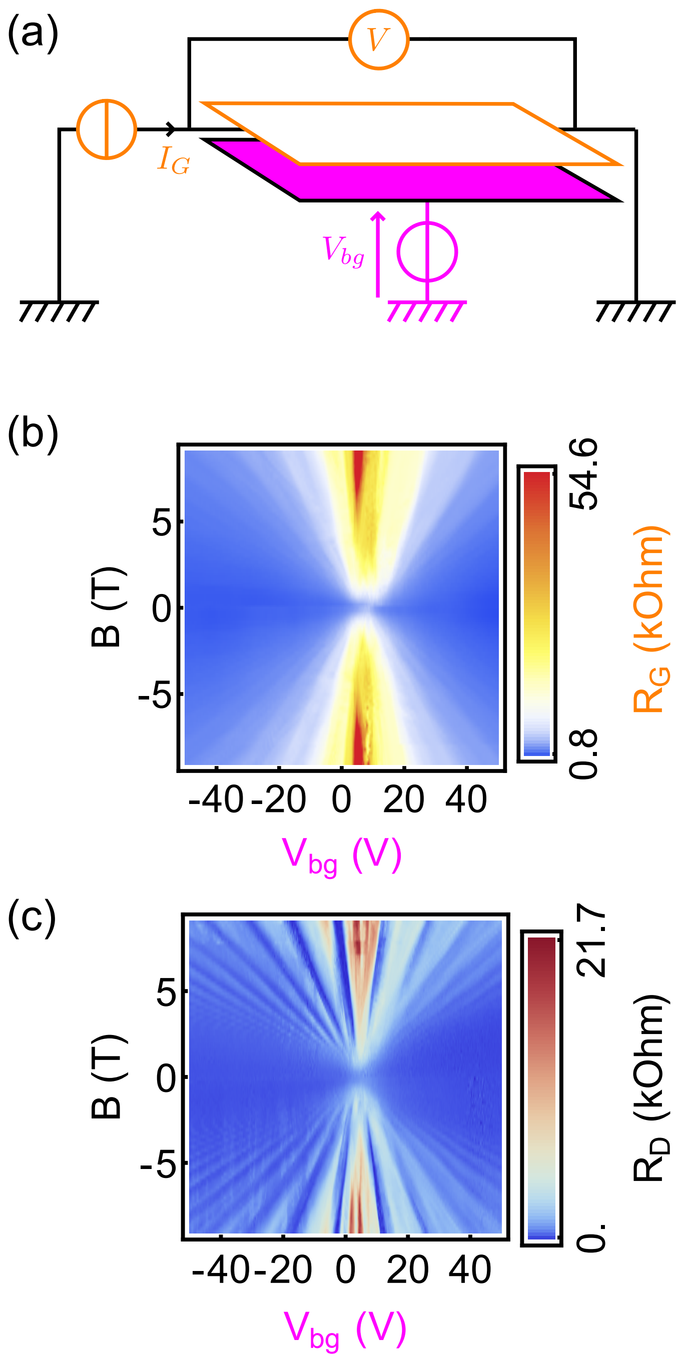


Figure S9. Onsager relation. (a) Setup for two-terminal measurement of the graphene resistance. (b) Two-terminal measurement of the graphene resistance $R_G$ as a function of $V_{bg}$ and $B$. It is symmetric with magnetic field and obeys Onsager relation. (c) Symmetrized drag resistance $R_D = \left(R_D^{NT}(B) + R_D^{G}(-B)\right)/2$ obtained from data of Fig 2 (d) and (e) of the main text. It is also symmetric with $B$ and fulfills the condition $R_D(B) = R_D(-B)$.

$R_D = \left(R_D^{NT}(B) + R_D^{G}(-B)\right)/2$ where $R_D^{NT(G)}$ is the drag resistance measured across the nanotube (resp. graphene).

## VI. MAGNETIC FIELD DEPENDENCE OF $R_D$

In Fig. 2d of the main text, we observe the formation of Landau levels. It is also clear that $R_D$ is increasing with magnetic field when averaged over a wide range of $V_{bg}$.

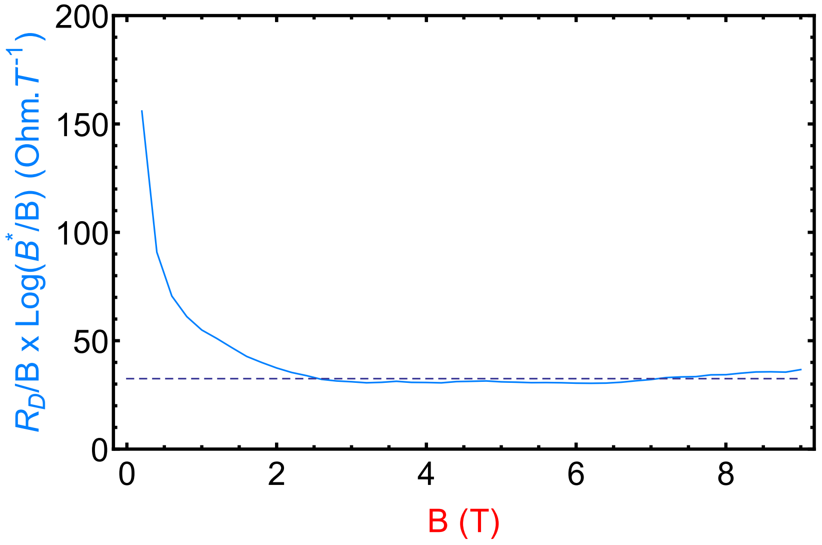


Figure S10. Normalized drag resistance $R_D$ as a function of magnetic field. $R_D$ has been averaged between -50 V and +50 V in order to average out the quantum Hall oscillations. $B^*$ is a constant giving an upper bound for the magnetic field beyond which the law $B \times \log(B^*/B)$ is not valid anymore. Here we take $B^* \approx 100$ T.

It is interesting to compare our measurements with predictions that have been made in the Quantum Hall regime for a system made of two 2D electron gases. Coulomb drag resistance is then expected to evolve with magnetic field [9] following power laws. As our measurements are performed at 1.6K, we are in the low temperature regime ($T \ll \Delta$ where $\Delta$ is the Landau levels broadening, typically of a few meV or equivalently tens of K) and it is predicted that $R_D$ should follow a $B \times \log(B^*/B)$ law. Fig. S10 shows the magnetic field dependence of $R_D$ normalized by $B \times \log(B^*/B)$ and averaged over a window of 100 V of back gate voltage $V_{bg}$ much larger than the Landau level spacings. We see that, beyond 2T, it is indeed constant with less than 10% deviation.

## VII. QUANTUM DOT WITH PHENOMENOLOGICAL FRICTION FORCE

In measurements of Fig. 3 (b) shown in the main text, we observe that charge fluctuations in the nanotube can dramatically affect the drag in the configuration where one electrode is grounded (right on Fig. 3 c) and the other one is floating (left) acquiring a potential $V_{NT}$. This behavior can be described by a phenomenological model where the nanotube is modeled as a quantum dot and the electrons that it contains experience a friction force. This force, proportional to the current $I_G$ flowing in the graphene flake, can be written $\vec{F}_f = \eta_{eff} I_G \vec{u}_{NT}$ where $\eta_{eff}$ is an effective friction coefficient and $\vec{u}_{NT}$ is a unitary vector along the carbon nanotube oriented in the positive direction of $I_G$. This friction force can displace electron between the grounded electrode and the floating one (Fig. 3 c and d) and therefore affect the potential $V_{NT}$ and the average number of charge $n_{NT}$ in the nanotube. If the distance between the source and drain electrodes connecting the nanotube is $L$, then the work $W_F$ of the friction force when an electron is transferred form source to drain is

$$W_F = \eta_{eff} I_G L$$

However, supposing that the device is approximately symmetric, an electron that stops in the nanotube will acquire a work $W_F/2$ because it travels only half the distance.

When no current is flowing through the graphene, the whole system is at equilibrium with $n_0$ charge in the nanotube (controlled by the back gate with a leverage $\alpha$) and a potential $V_{NT} = 0$ on the floating electrode. If $I_G \neq 0$, then the system is driven out-of-equilibrium and a given number of electron $N$ is transferred from the grounded to the floating electrode while the average number of charge in the nanotube changes by an amount $\delta n_{NT} = n_{NT} - n_0$. The potential of the floating electrode $V_{NT}$ therefore becomes finite and, supposing the device is approximately symmetric, the potential of the nanotube changes as well to $V_{NT}/2$. The energy of the whole system thus increases by

$$\Delta E(N, \delta n_{NT}) = -e(N \times V_{NT} + n_{NT} \times V_{NT}/2) + (N \times W_F + \delta n_{NT} \times W_F/2) + \frac{e^2}{2C_{NT}}\left[(n_{NT} - \alpha V_{bg})^2 - (n_0 - \alpha V_{bg})^2\right]$$

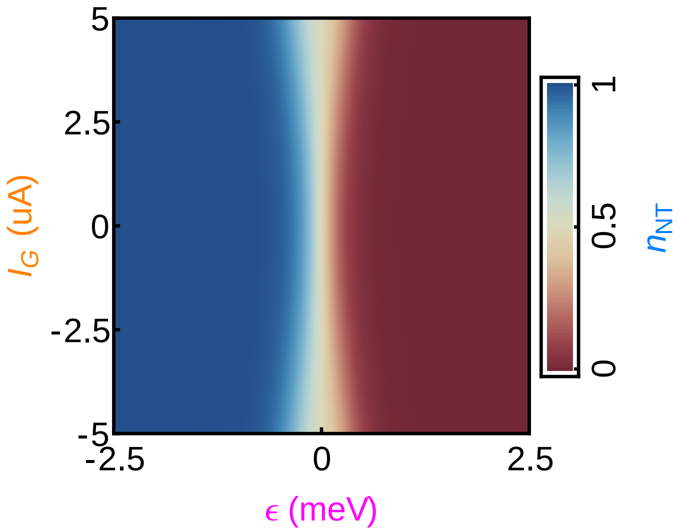


Figure S11. Calculation of charge fluctuations calculated from Eq. 2. The charge in the quantum dot is controlled by the back gate that controls the energy of the orbital $\epsilon$. The current flowing through the graphene can also induces fluctuations that we can see as the white areas, corresponding to $n_{NT} = 0.5$, expands.

where the first term is the change of electrostatic energy due to the increase of $V_{NT}$, the second is the work of the friction, and the third one is the variation of charging energy of the nanotube, $C_{NT}$ being the capacitance of the nanotube. Here, we have neglected the charging energy of the floating electrode since its capacitance (hundreds of fF, essentially due to the wiring) is typically 3 orders of magnitude large than $C_{NT}$ (hundreds of aF).

For a given $I_G$, the minimum energy of the system is reached for $\partial \Delta E / \partial \delta n_{NT} = 0$ which leads to the equality

$$V_{NT} = \frac{\eta_{eff} L}{e} I_G + 2e \frac{\delta n_{NT}}{C_{NT}} \tag{1}$$

The drag resistance is thus given by $R_D = \partial V_{NT} / \partial I_G$, and we can introduce a constant $R_D^0 = \eta_{eff} L / e$ that is the drag resistance if we neglect the charge fluctuations. In Fig. 3 (b), $R_D^0$ corresponds to $R_D$ measured at $I_G = 0$ and is approximately equal to 125Ω for this range of $V_{bg}$.

The role of $\delta n_{NT}$ can be taken into account modeling the carbon nanotube as a quantum dot and considering only a single orbital of energy $\epsilon$, tunable linearly with $V_{bg}$, that is the closest to the Fermi energy of the electrodes. We consider here the simplest case of a single energy level with a sufficiently large charging energy $e^2/C_{NT}$ such that this orbital can only be unoccupied or singly occupied, with a small symmetric coupling $\Gamma \ll k_B T$ to the two electrodes ($k_B$ is the Boltzmann constant and $T$ the temperature). Under these conditions, one can calculate the average charge in the quantum dot by solving master equations of the system [10]

$$\delta n_{NT} = \frac{1}{2\left(\exp\left(\frac{\mu_{NT} - \mu_L}{k_B T}\right) + 1\right)} + \frac{1}{2\left(\exp\left(\frac{\mu_{NT} - \mu_R}{k_B T}\right) + 1\right)} \tag{2}$$

where $\mu_{NT} = \epsilon - eV_{NT}/2$, $\mu_R = -eV_{NT}$ and $\mu_L = 0$. In principle, one should solve the problem self-consistently on $\delta n_{NT}$ combining Eq. 1 and 2. For simplicity, we calculate $V_{NT}$ at first order in the fluctuations ($\delta n_{NT} \ll 1$) taking $\mu_R \approx -W_F$ and $\mu_{NT} \approx \epsilon - W_F/2$. Fig. S11 shows that $\delta n_{NT}$ can be controlled with the back gate ($\epsilon \propto -V_{bg}$) but also with the current $I_G$ flowing through graphene.

Similarly, we can calculate the conductance of the nanotube $G_{NT}$ with the master equation formalism. If we consider this time that one electrode is grounded and the other one is connected to a voltage source applying a voltage $V_{bias}$, then the current flowing through the nanotube for $I_G = 0$ is given by

$$I_{NT} = \frac{4e\Gamma}{h} \left[ \frac{1}{\left(\exp\left(\frac{\epsilon_0 - eV_{bias}/2}{k_B T}\right) + 1\right)} - \frac{1}{\left(\exp\left(\frac{\epsilon_0 + eV_{bias}/2}{k_B T}\right) + 1\right)} \right]$$

The nanotube conductance is given by $G_{NT} = \partial I_{NT} / \partial V_{bias}$. In Fig. S12, we can see that $G_{NT}$ is peaked when the Fermi level of source or drain is aligned with $\epsilon$. The peaks have a half width at half maximum (HWHM) given by the

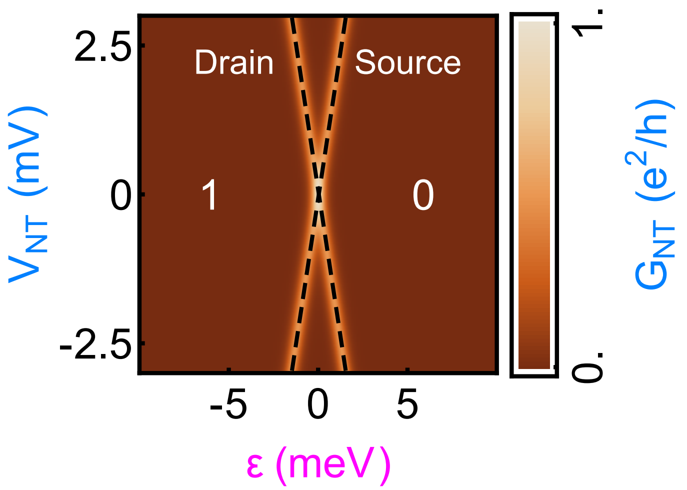


Figure S12. Calculation of Coulomb diamonds. The number of charge $n_{NT}$ is indicated in each diamonds.

temperature $k_BT/e$ provided that $\Gamma \ll k_BT$. If $\Gamma \gtrsim k_BT$, then the width is given by $\Gamma$ and one can then replace $T$ by an effective temperature $T_{eff} = \Gamma/k_B$.

In Fig. 3h the main text, we obtain the simulated drag resistance of Fig. 3 choosing $R_D^0 = 125\ \Omega$, $C_{NT} = 16$ aF and $\Gamma = 0.35$ meV (measured through HWHM of conductance peaks in $G_{NT}$ shown in Fig. 3g) which gives a reasonable agreement with our observations. This value of $C_{NT}$ is consistent with the typical charging energy that we observe ($\approx 10$ meV).

## VIII. EVALUATION OF THE FRICTION COEFFICIENT

Within the friction force model that we present above, we can try to give an estimation for the friction constant $\eta$ from our experimental observations.

We have define the friction force as

$$\vec{F}_{friction} = \eta n_G \vec{v}$$

where $\eta$ is the friction coefficient, $\vec{v}$ is the average velocity of charge carriers in graphene and $n_G$ is the carrier concentration.

For an homogenous current $I_G$ over the graphene flake, we have $I_G = e n_G \vec{v} \times W_G$ where $e$ is the electron charge and $W_G$ the width of the graphene flake. We can therefore introduce an effective friction coefficient $\eta_{eff}$ to relate this force to the current flowing in graphene $I_G$

$$F = \eta_{eff} I_G$$

with

$$\eta_{eff} = \frac{\eta}{e \times W_G}$$

In previous section, we saw that we can relate this coefficient to the average drag resistance

$$R_D = \frac{\eta_{eff} L}{e}$$

where $L$ is the length of the nanotube. From this, we can write

$$\eta = \frac{R_D e^2 W_G}{L}$$

which gives

$$\eta \approx 1.9 \times 10^{-34}\ \text{J.s}$$

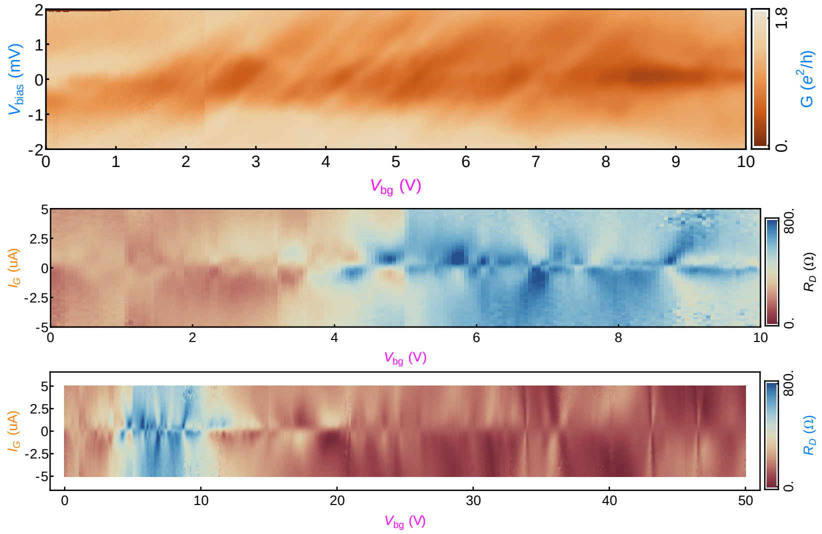


Figure S13. From top to bottom. Nanotube conductance measured at finite bias voltage $V_{bias}$ across the nanotube as a function of $V_{bg}$. Drag resistance $R_D$ measured out-of-equilibrium in the same back gate voltage range. $R_D$ measured for $V_{bg}$ between 0 and 50 V at finite current in the graphene flake $I_G$.

for $R_D = 750\ \Omega$ (value at the Dirac peak), $W_G = 10\ \mu$m and $L = 1\ \mu$m. Expressed in unit of $\hbar$, this gives

$$\eta \approx 1.8\hbar$$

This estimation is very rough as it supposed an homogenous current in the graphene flake which is clearly not the case in our sample.

It is interesting to compare this estimation with what has been observed and predicted for graphene-graphene devices [11]. In that case, the friction coefficient can be expressed as [12]

$$\eta_G = \alpha^2 \hbar$$

where the interaction strength $\alpha = 0.25$. This gives $\eta_G \approx 6.5 \times 10^{-36}$, an order of magnitude lower than our estimation. In our nanotube-graphene device, the equivalent interaction strength would be $\alpha = 1.3$ suggesting that interaction are more proeminent.

## IX. OUT-EQUILIBRIUM DRAG RESISTANCE MEASURED AT LOW GATE VOLTAGE

In Fig. 3 of the main text, we present measurements of drag resistance, for back gate voltage larger than 30 V, when the nanotube is in the Coulomb blockade regime. In this regime, we observe correlations between patterns observed in $R_D$ measured out-of-equilibrium and the nanotube conductance $G_{NT}$. These patterns are well defined because of the strong non-linearity related to Coulomb blockade.

However, at lower gate voltage, the carbon nanotube is not in the Coulomb blockade regime and the conductance evolves very smoothly with $V_{bg}$ as can be expected from a metallic nanotube. Fig. S13 shows nanotube conductance measurement as a function of $V_{bg}$ between 0 and 10 V and the conductance oscillates smoothly suggesting that the nanotube is in the Fabry-Perot regime with irregularities likely due to disorder induced by resist residue. In that regime, though $R_D$ shows similar out-of-equilibrium modulation, the correlations between $R_D$ and $G_{NT}$ are not as obvious since there is no characteristic patterns that emerges over the background. The bottom graph of Fig. S13 shows the evolution of $R_D$ measured out-of-equilibrium from the Fabry-Perot regime for $V_{bg}$ below 30V to the Coulomb blockade regime above 30 V.

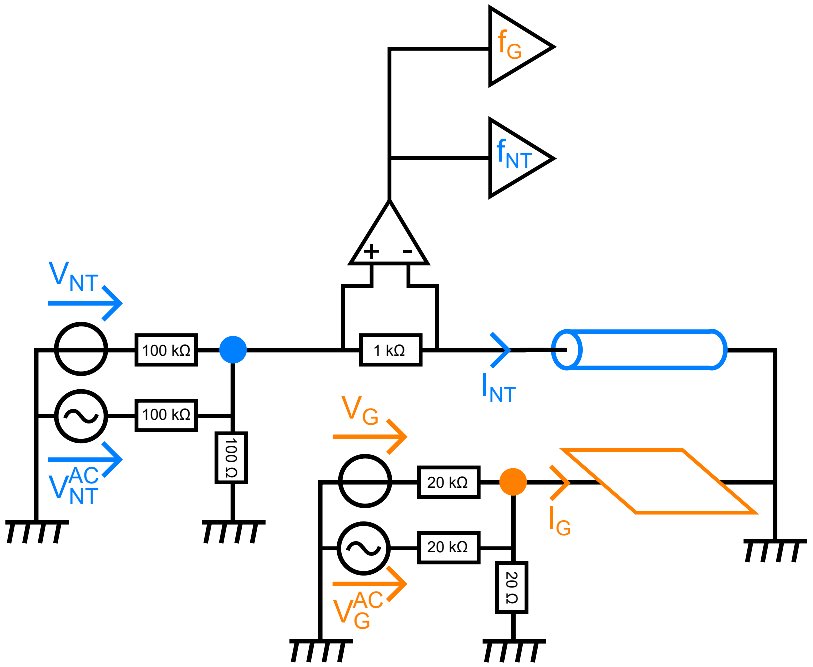


Figure S14. Setup for simultaneous measurement of $G_{NT}$ and $R_D$. Voltages are applied across the nanotube and graphene. Using voltage dividers, AC and DC parts are summed such that on the blue (resp. orange) spot the total voltage that is applied is $V_{NT}^{tot} = \left(V_{NT} + V_{NT}^{AC}\cos\left(2\pi f_{NT} t\right)\right)/1000$ (resp. $V_G^{tot} = \left(V_G + V_G^{AC}\cos\left(2\pi f_G t\right)\right)/1000$). Using a differential voltage amplifier, we measure the current $I_{NT}$ flowing through the nanotube that we deduce from the voltage across a resistance of 1k$\Omega$, negligible compared to $R_{NT}$ , in series with the nanotube. Two lock-in amplifiers are measuring at frequencies $f_G$ and $f_{NT}$ the differential conductance of the nanotube $G_{NT}$ and the differential drag conductance $\sigma_D$.

## X. LINEAR LUMPED ELEMENT ANALYSIS AND SETUP FOR SIMULTANEOUS MEASUREMENT OF $G_{NT}$ AND $R_D$

### A. Setup for simultaneous measurement of $G_{NT}$ and $R_D$

Measurements presented in Fig. 4 of the main text are obtained by applying voltages at the same time on nanotube ($V_{NT}$) and graphene ($V_G$). This way, we get a current $I_{NT}$ through the nanotube with two components: a standard resistive contribution due to $V_{NT}$ and a drag contribution due to $V_G$. We can distinguish these two contributions by frequency-division multiplexing using the setup of Fig. S14 with voltages having both a DC and an AC part and using two lock-in amplifiers set at different frequency $f_{NT}$ and $f_G$ respectively for $V_{NT}$ and $V_G$.

### B. Linear lumped element analysis

Fig. 4 (c) of the main text shows measurements of $R_D$ as a function of voltages applied across the nanotube $V_{NT}$ and the graphene flake $V_G$ (see Fig. 4 (a)). In this configuration, none of the electrodes are floating and uncontrolled charge fluctuations are suppressed. However, we can see that $R_D$ is not a constant in the $(V_{NT}, V_G)$ plane, it can even cancel and take negative values. It is instructive to perform a linear lumped element analysis of the device in order to extract information about its behavior.

The simplest description of the charge drag we can do is to consider that the nanotube (resp. the graphene) behaves as a voltage source whose electromotive force $R_D I_G$ (resp. $R_D I_{NT}$) is driven by the current flowing in the graphene (resp. nanotube). This source has a series resistance corresponding to the resistance of the nanotube $R_{NT}$ (resp. graphene $R_G$) in absence of drag. The configuration of Fig. 4 (a) is thus equivalent to the schematic of Fig. 4 (b) from which we can write

$$\begin{cases} V_{NT} - R_D I_G & = R_{NT} I_{NT} \\ V_G - R_D I_{NT} & = R_G I_G \end{cases}$$

If we combine this two coupled equations, we find that

$$I_{NT} = \frac{R_G}{R_{NT}R_G + R_D^2}\left[V_{NT} - \frac{R_D}{R_G}V_G\right]$$

As in our case $R_D, R_G \ll R_{NT}$, we get

$$\begin{cases} \partial I_{NT}/\partial V_{NT} & \approx 1/R_{NT} \\ \partial I_{NT}/\partial V_G & \approx R_D/R_G R_{NT} \end{cases}$$

that we can respectively define as the nanotube conductance $G_{NT}$ and the drag conductance $\sigma_D$. We get the drag resistance using the relation $R_D = \sigma_D R_G R_{NT}$.

We can also identify regions where currents in the nanotube and graphene are in similar or opposite directions. If we set $I_G = 0$, we get $V_G = R_D/R_{NT}V_{NT}$, therefore if $V_G > R_D/R_{NT}V_{NT}$ (resp. $V_G < R_D/R_{NT}V_{NT}$) then $I_G > 0$ (resp. $I_G < 0$). As $R_D \ll R_{NT}$, this limit is roughly $V_{NT} \approx 0$. Similarly, if we set $I_{NT} = 0$, we get $V_{NT} = R_D/R_G V_G$ and we can identify where $I_{NT}$ is positive or negative. These two boundaries are represented by dotted line in Fig. 4 (c) of the main text.

## XI. TEMPERATURE AND CARRIER DENSITY DEPENDENCES IN ADDITIONAL DEVICES

The device presented in the manuscript is the one in which we detected the larger signal when measuring the drag resistance. This might be because of the proximity of the nanotube to the graphene electrode used to drain the current therefore maximizing the amount of current actually flowing below the nanotube. In other samples, designed in different geometries with graphene electrical contacts further from the position of the nanotube, we measured drag resistance that were smaller by one or two orders of magnitude. They also show strong dependences with temperature, charge carrier density and magnetic field.

Fig. S15 shows the temperature dependence of $R_D$ for two other devices (2 and 3). Device 2 shows a drag resistance $R_D$ with the same sign than the device we present in the main part of the manuscript and also seems to diverge at low temperature, though the variation is much smaller. In device 3, $R_D$ was very small at large temperature but started to become measurable close to 10 K and below. The magnitude of $R_D$ was increasing with decreasing temperature but could be positive or negative depending on the potential of the nanotube with respect to the graphene flake (in this sample nanotube and graphene did not share a common electrode and it was therefore possible to have them at different potential).

In Fig. S16, we show measurement of $R_D$ in device 3' (circuits 3 and 3' were part of the same electrical device, they shared the same graphene flake but $R_D$ was not measured across the same section of nanotube) as a function of magnetic field and back gate voltage. It shows the same fan structure as for the device presented in the main part of the manuscript except that $R_D$ can take negative values rather than cancelling when the Fermi level of graphene is in between Landau levels. However, given the magnitude of the signal we measured (only a few Ohms), it is very likely that a significant part of this signal is due to capacitive cross-talk between nanotube and graphene that can induce a negative contribution in the signal. This hypothesis is supported by the fact that in this device, Onsager relations were violated when the role of nanotube and graphene were inverted.

Fig. S17 shows a comparison of out-of equilibrium measurements between this device and the one presented in the main text. Though the evolution with $V_{bg}$ is not as regular, probably due to additional parasitic capactive signal, we observe a similar behavior with a drag resistance $R_D$ which can increase or decrease depending on $I_G$.

---

[1] L. Wang, I. Meric, P. Y. Huang, Q. Gao, Y. Gao, H. Tran, T. Taniguchi, K. Watanabe, L. M. Campos, D. A. Muller, J. Guo, P. Kim, J. Hone, K. L. Shepard, and C. R. Dean, Science **342**, 614 (2013).
[2] M. Y. Sfeir, F. Wang, L. Huang, C.-C. Chuang, J. Hone, S. P. O'Brien, T. F. Heinz, and L. E. Brus, Science **306**, 1540 (2004).
[3] X. M. H. Huang, R. Caldwell, L. Huang, S. C. Jun, M. Huang, M. Y. Sfeir, S. P. O'Brien, and J. Hone, Nano Letters **5**, 1515 (2005).
[4] D. Laroche, G. Gervais, M. P. Lilly, and J. L. Reno, Science **343**, 631 (2014).
[5] L. Onsager, Physical Review **37**, 405 (1931).
[6] M. Büttiker, Physical Review Letters **57**, 1761 (1986).
[7] A. F. Croxall, K. Das Gupta, C. A. Nicoll, M. Thangaraj, H. E. Beere, I. Farrer, D. A. Ritchie, and M. Pepper, Physical Review Letters **101**, 246801 (2008).

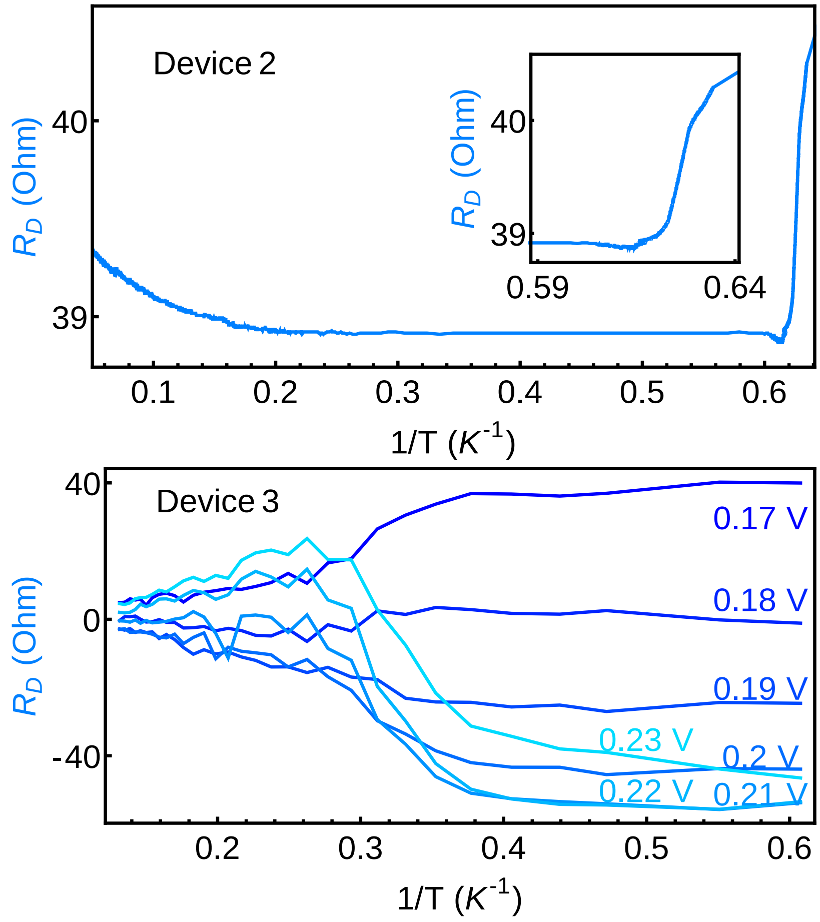


Figure S15. Drag resistance $R_D$ measured across the carbon nanotube in additional devices 2 (top) and 3 (bottom) as a function of the inverse of temperature $1/T$. In device 2, $R_D$ decrease slowly from 15 K to 2 K and then experiences a sharp increase close to 1.6 K. The inset shows a zoom on this increase. In device 3, nanotube and graphene did not share a common electrode, it was therefore possible to apply a voltage on the nanotube to change its potential with respect to the graphene flake. Depending on this potential (values given in the graph), $R_D$ would take negative or positive values with an increasing magnitude for decreasing temperature.

[8] S. Kim and E. Tutuc, Solid State Communications Exploring Graphene, Recent Research Advances, **152**, 1283 (2012).
[9] I. V. Gornyi, A. D. Mirlin, and F. von Oppen, Physical Review B **70**, 245302 (2004).
[10] C. W. J. Beenakker, Physical Review B **44**, 1646 (1991).
[11] M. Titov, R. V. Gorbachev, B. N. Narozhny, T. Tudorovskiy, M. Schütt, P. M. Ostrovsky, I. V. Gornyi, A. D. Mirlin, M. I. Katsnelson, K. S. Novoselov, A. K. Geim, and L. A. Ponomarenko, Physical Review Letters **111**, 166601 (2013).
[12] J. C. W. Song, D. A. Abanin, and L. S. Levitov, Nano Letters **13**, 3631 (2013).

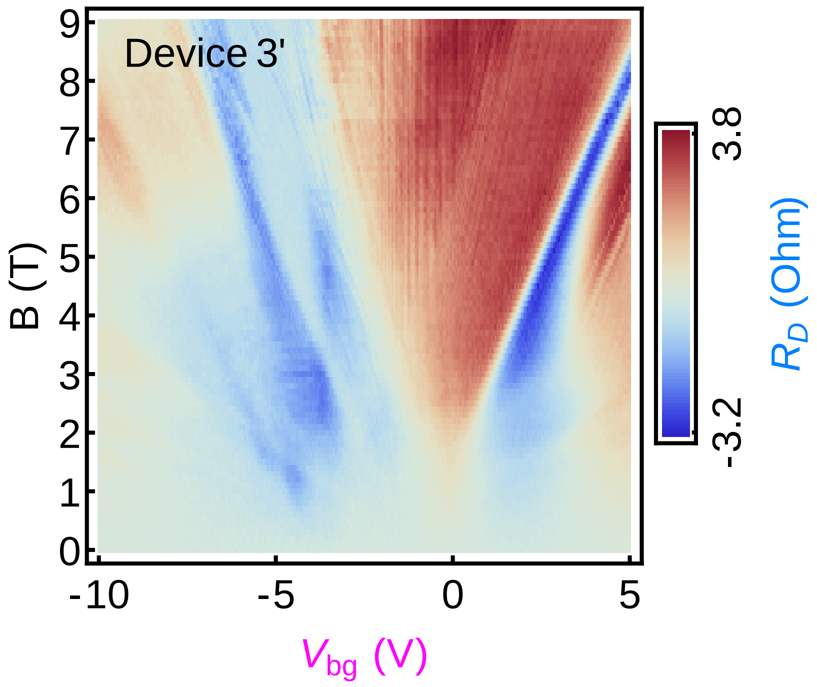


Figure S16. Drag resistance measured across the carbon nanotube as a function of magnetic field $B$ and back gate voltage $V_{bg}$ in device 3'. Both nanotube and graphene were connected to the ground.

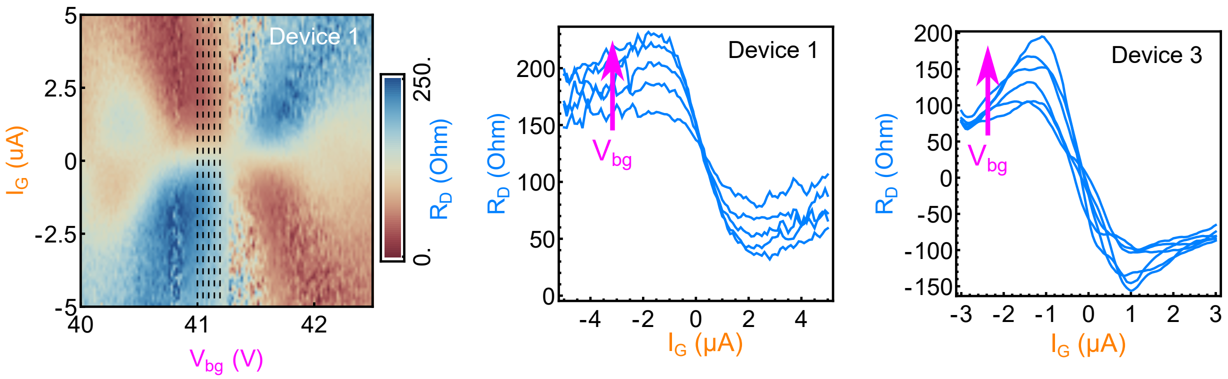


Figure S17. Outof-equilibrium measurements performed in device 1 and 3. The left graph shows a zoom on Fig. 3b of the main text and the black dashed lines indicate where cut of the graph in the center has been taken. These cuts are compared with measurements of $R_D$ taken in device three (right) as a function of $I_G$ for different voltages applied on the back gate.
